# Supplementary material for: Understanding Certified Training with Interval Bound Propagation
Source: arXiv:2306.10426 source file (2026-10-31)
Supplement: Supplementary file 1 [file appendix_eval.tex]

\section{Extended Evaluation}

\paragraph{TAPS Accuracy as GoF}
In practice, we want to avoid certifying every model with expensive certification methods, especially during hyperparameter tuning and applying early stopping. Therefore, we need a criterion to select models. In this section, we aim to show that TAPS accuracy is a good instrument for GoF.

We compare the TAPS accuracy to adversarial and certified accuracy with all models we get on MNIST and CIFAR-10. The result is shown in \cref{tb:TB_adv_cert}. From \cref{tb:TB_adv_cert}, we can see that the correlations between TAPS accuracy and both the adversarial and the certified accuracy are close to 1. In addition, the differences are small and centered at zero, with a small standard deviation. Therefore, we conclude that TAPS accuracy is a good estimation of the true robustness, thus a good measurement of GoF. In all the experiments, we perform model selection based on the TAPS accuracy.

\begin{table}
    \caption{Comparasion of TAPS accuracy with certified and adversarial accuracy.} 
    \label{tb:TB_adv_cert}
    \resizebox{0.98\linewidth}{!}{
        \begin{tabular}{ccccc} \toprule
            \textbf{Dataset}  & \textbf{cor(T.B., cert.)} & \textbf{cor(T.B., adv.)} & \textbf{T.B. $-$ cert.} & \textbf{T.B. $-$ adv.} \\ \midrule
            \textbf{MNIST}    & 0.9139                    & 0.9633                   & 0.0122 $\pm$ 0.0141     & 0.0033 $\pm$ 0.0079    \\
            \textbf{CIFAR-10} & 0.9973                    & 0.9989                   & 0.0028 $\pm$ 0.0095     & -0.0040 $\pm$ 0.0077   \\ \bottomrule
        \end{tabular}
    }
\end{table}

\paragraph{Training Difficulty}

Since TAPS is merely a training technique, we can test TAPS-trained models trained with a new classifier split. By design, if the training is successful, then under a given classifier split for testing, the model trained with the same split should have the best TAPS accuracy. Although this is often true, we find that in some cases, a smaller classifier split results in higher TAPS accuracy, indicating the difficulty of training.

\cref{fig:trainability_cifar} shows the tested TAPS accuracy for models trained with IBP and different splits for CIFAR-10. The result on MNIST is provided in \cref{fig:trainability_mnist}. From these figures, we can see that for CIFAR-10 $\epsilon=2/255$ and MNIST, the models trained with the same test split has the highest TAPS accuracy, as expected. However, for CIFAR-10 $\epsilon=8/255$, the model trained with classifier size 4 is consistently better for all test splits. Furthermore, as we show in \cref{sec:split}, this model has the best adversarial and certified accuracy as well. This means that in this setting, the training of larger splits is too difficult, such that TAPS is not able to find a good model to minimize the given loss. However, in other settings, TAPS is easy enough to train.
\begin{figure}
    \centering
    \includegraphics[width=.9\linewidth]{figures/cifar10_eps2.255_training_quality.pdf}
    \includegraphics[width=.9\linewidth]{figures/cifar10_eps8.255_training_quality.pdf}
    \caption{TAPS accuracy of models trained by different classifier size. The top subfigure is on CIFAR-10 $\epsilon=\frac{2}{255}$; the bottom subfigure is on CIFAR-10 $\epsilon=\frac{8}{255}$.}
    \label{fig:trainability_cifar}
\end{figure}

\begin{figure}[h]
    \centering
    \includegraphics[width=.9\linewidth]{figures/mnist_eps0.1_training_quality.pdf}
    \includegraphics[width=.9\linewidth]{figures/mnist_eps0.3_training_quality.pdf}
    \caption{TAPS accuracy of models trained by different classifier size. The top subfigure is on MNIST $\epsilon=0.1$; the bottom subfigure is on MNIST $\epsilon=0.3$.}
    \label{fig:trainability_mnist}
\end{figure}

\paragraph{Split Position}

We include the full tables of the experiment in \cref{sec:split} in \cref{tb:abalation_classifier_size_mnist} and \cref{tb:abalation_classifier_size_cifar}.
\begin{table}
    \centering
    \caption{Effect of split position into the classifier and feature extractor (overall model size remains unchanged). All numbers are in percentages. All results for \mnist.}
    \label{tb:abalation_classifier_size_mnist}
    \vspace{5pt}
    \resizebox{0.98\linewidth}{!}{
        \begin{tabular}{cccccccc}
            \toprule
            \multirow{2.5}{*}{$\epsilon$} & \multirow{2.5}{*}{{Classifier size}} & \multirow{2.5}{*}{{Nat.}} & \multirow{2.5}{*}{{Adv.}} & \multicolumn{4}{c}{{Cert.}}\\
            \cmidrule(lr){5-8}
            &&&& {Total}& {IBP} & {C-IBP} & {MN-BaB} \\ 
            \midrule
            \multirow{7}{*}{0.1} & IBP & 98.87& 98.16& 98.13& 97.83& +0.17& +0.13 \\
            & 4 & 99.06& 98.37& 98.31& 96.27& +1.52& +0.52 \\
            & 8 & 99.16& 98.35& 98.25& 87.82& +8.11& +2.32 \\
            & 11& 99.19& \textbf{98.51}& \textbf{98.39}& 62.83& +27.34 & +8.22 \\
            & 14& \textbf{99.28}& 98.47& 98.03& 4.75 & +47.25 & +46.03\\
            & 17& 99.22& \textbf{98.51}& 98.17& 9.76 & +53.32 & +35.09\\
            & 20& 99.09& 98.45& 98.27& 81.89& +12.62 & +3.76 \\ 
            \cmidrule(lr){1-8}
            \multirow{7}{*}{{0.3}} & IBP & 97.60& 93.37& 93.15& 93.08& +0.03& +0.04 \\
            & 4 & 97.94& 94.01& \textbf{93.62}& 92.76& +0.55& +0.31 \\
            & 8 & 98.16& 94.18& 93.55& 91.85& +0.87& +0.83 \\
            & 11& 98.63& 94.48& 93.03& 89.40& +1.60& +2.03 \\
            & 14& 98.7 & 94.85& 93.44& 89.52& +1.83& +2.09 \\
            & 17& 98.63& 94.64& 93.26& 89.15& +1.98& +2.13 \\
            & 20& \textbf{98.88}& \textbf{95.11}& 92.70& 85.03& +3.61& +4.06 \\
            \bottomrule
        \end{tabular}
    }
\end{table}

\begin{table}
    \centering
    \caption{Effect of split position into the classifier and feature extractor (overall model size remains unchanged). All numbers are in percentages. All results for \cifar.}
    \label{tb:abalation_classifier_size_cifar}
    \vspace{5pt}
    \resizebox{0.98\linewidth}{!}{
        \begin{tabular}{ccccccc}
            \toprule
            \multirow{2.5}{*}{$\epsilon$} & \multirow{2.5}{*}{{Classifier size}} & \multirow{2.5}{*}{{Nat.}} & \multirow{2.5}{*}{{Adv.}} & \multicolumn{3}{c}{{Cert.}}\\
            \cmidrule(lr){5-7}
            &&&& {Total}& {IBP} & {MN-BaB} \\ 
            \midrule
            \multirow{7}{*}{{2/255}} & IBP & 67.27& 56.32& 56.14& 53.54& +2.60 \\
            & 4 & 70.10& 57.78& 57.48& 41.86& +15.62 \\
            & 8 & 70.74& 57.83& 57.39& 40.24& +17.25 \\
            & 11& 71.88& 58.89& 58.23& 34.41& +23.82 \\
            & 14& 72.45& 60.38& 59.47& 31.88& +27.59\\
            & 17& 75.09& \textbf{63.00}& \textbf{61.56}& 24.36& +37.20\\
            & 20& \textbf{75.40}& 62.73& 61.11& 24.90& +36.21\\ 
            \cmidrule(lr){1-7}
            \multirow{7}{*}{{8/255}} & IBP & 48.15& 34.63& 34.60& 34.26& +0.34 \\
            & 4 & 49.76& \textbf{35.29}& \textbf{35.10}& 32.92& +2.18 \\
            & 8 & 47.28& 33.54& 33.12& 28.94& +4.18 \\
            & 11& 48.76& 33.50& 33.12& 29.14& +3.98 \\
            & 14& 50.19& 34.78& 34.35& 29.14& +5.21 \\
            & 17& 50.2 & 34.33& 33.72& 28.83& +4.89 \\
            & 20& \textbf{51.03}& 35.25& 34.44& 29.97& +4.47 \\
            \bottomrule
        \end{tabular}
    }
\end{table}

\paragraph{Tightness Coefficient for Different Width}

We repeat our experiment in \cref{sec:empirical_PI} for fully connected 3-layer network with different width and show the result in \cref{fig:PIC_width}. The narrow and wide network has $1/4$ and $4$ times of the width of the medium network, respectively. \cref{sec:empirical_PI} shows the trend is consistent for all the models, further supporting our discussion in \ref{sec:empirical_PI}. In addition, \cref{sec:empirical_PI} shows that larger networks, thus having more capacity, requires less propagation invariance. This suggests that larger models are able to handle the additional regularization introduced by spurious points and thus need less propagation invariance.
